# Supplementary material for: Optimal Transport-Based Displacement Interpolation with Data Augmentation for Reduced Order Modeling of Nonlinear Dynamical Systems
Source: arXiv:2411.08750 source file (2024-11-13)
Supplement: Supplementary file 1 [file appendix.tex]

\appendix
\section{Gaussian Process Regression}
\label{app:gpr}

Gaussian Process (GP) regression is a powerful, non-parametric Bayesian approach to modeling complex functions. Unlike traditional regression methods that assume a specific functional form, GP regression models the distribution over potential functions, offering greater flexibility and the ability to capture intricate patterns in data.

% \subsection{Fundamentals of Gaussian Processes}
A Gaussian Process is defined as a collection of random variables, any finite number of which have a joint Gaussian distribution. In a regression task, we model a function $f$ as the GP:
\begin{equation}
    f(\boldsymbol{\mu}) \sim \mathcal{GP}(m(\boldsymbol{\mu}), \kappa(\boldsymbol{\mu}, \boldsymbol{\mu}')),
\end{equation}
where $\boldsymbol{\mu} \in \mathcal{P}$ is an input vector, $m(\boldsymbol{\mu})$ is the mean function, representing our prior belief about its behavior, and $\kappa(\boldsymbol{\mu}, \boldsymbol{\mu}')$ is the covariance function (or kernel), encoding the similarity between function values at different input points.

% \subsection{Gaussian Process Regression Model}
Given a set of $N$ training inputs $\mathbf{X} = [\boldsymbol{\mu}^1, \boldsymbol{\mu}^2, \ldots, \boldsymbol{\mu}^N]$ and corresponding outputs $\mathbf{y} = [y_1, y_2, \ldots, y_N]^T$, GP regression models the joint distribution of the observed data and predictions for new testing inputs $\mathbf{X}_*$ as the multivariate Gaussian:
\begin{equation}
    \begin{bmatrix}
        \mathbf{y} \\
        \mathbf{f}_*
    \end{bmatrix} \sim \mathcal{N}\left(
    \begin{bmatrix}
        \mathbf{m} \\
        \mathbf{m}_*
    \end{bmatrix},
    \begin{bmatrix}
        \mathbf{K} & \mathbf{K}_* \\
        \mathbf{K}_*^T & \mathbf{K}_{**}
    \end{bmatrix}
    \right)
\end{equation}
where:
\begin{itemize}
    \item $\mathbf{m} = m(\mathbf{X})$ is the mean functions evaluated at training  points.
    \item $\mathbf{m}_* = m(\mathbf{X}_*)$ is the mean functions evaluated at testing points.
    \item $\mathbf{K} = \kappa(\mathbf{X}, \mathbf{X})$ is the covariance matrix between training points.
    \item $\mathbf{K}_* = \kappa(\mathbf{X}, \mathbf{X}_*)$ is the covariance matrix between training and testing points.
    \item $\mathbf{K}_{**} = \kappa(\mathbf{X}_*, \mathbf{X}_*)$ is the covariance matrix between testing points.
\end{itemize}

% \subsection{Prediction with Gaussian Processes}
The posterior distribution for predictions at new input points $\mathbf{X}_*$, given the training data, is derived using the properties of multivariate Gaussian distributions, for which one has the following formula:
\begin{equation}
    \mathbf{f}_* | \mathbf{X}, \mathbf{y}, \mathbf{X}_* \sim \mathcal{N}(\boldsymbol{\mu}_*, \boldsymbol{\Sigma}_*),
\end{equation}
where:
\begin{align}
    \boldsymbol{\mu}_* &= \mathbf{m}_* + \mathbf{K}_*^T \mathbf{K}^{-1} (\mathbf{y} - \mathbf{m}), \\
    \boldsymbol{\Sigma}_* &= \mathbf{K}_{**} - \mathbf{K}_*^T \mathbf{K}^{-1} \mathbf{K}_*.
\end{align}
This formulation provides both the mean prediction $\boldsymbol{\mu}_*$ and the uncertainty in the prediction $\boldsymbol{\Sigma}_*$, which is a key advantage of GP regression.

% \subsection{Covariance Functions}
The choice of covariance function is crucial in GP regression as it encodes our assumptions about the function we are modeling. A commonly used covariance function is the squared exponential (SE) kernel:
\begin{equation}
    \kappa_\text{SE}(\boldsymbol{\mu}, \boldsymbol{\mu}') = \sigma_f^2 \exp\left(-\frac{1}{2l^2}||\boldsymbol{\mu} - \boldsymbol{\mu}'||^2\right),
\end{equation}
where $\sigma_f^2$ is the signal variance and $l$ is the length scale. These hyperparameters control the amplitude and smoothness of the function, respectively.

% \subsection{Hyperparameter Optimization}
The performance of GP regression heavily depends on the choice of hyperparameters in the covariance function. These are typically optimized by maximizing the log marginal likelihood w.r.t.\ the hyperparameters $\boldsymbol{\theta}$:
\begin{equation}
    \log p(\mathbf{y}|\mathbf{X}, \boldsymbol{\theta}) = -\frac{1}{2}\mathbf{y}^T\mathbf{K}^{-1}\mathbf{y} - \frac{1}{2}\log|\mathbf{K}| - \frac{n}{2}\log(2\pi).
\end{equation}
% where  represents the . This optimization balances model fit against complexity, naturally implementing Occam's razor.
% \subsection{Advantages and Limitations}
GP regression offers several advantages:
\begin{itemize}
    \item Non-parametric flexibility to model complex functions.
    \item Built-in uncertainty quantification.
    \item Ability to incorporate prior knowledge through the mean and covariance functions.
\end{itemize}
However, it also comes with some limitations:
\begin{itemize}
    \item Computational complexity scales cubically with the number of data points.
    \item Difficulty in handling very large datasets.
    \item Sensitivity to the choice of covariance function and hyperparameters.
\end{itemize}

Despite these limitations, GP regression remains a powerful tool in many applications, particularly in scenarios with limited data or where uncertainty quantification is crucial.
